# Supplementary material for: Unsupervised Joint Learning of Optical Flow and Intensity with Event Cameras
Source: arXiv:2503.17262 source file (2025-07-22)
Supplement: Supplementary file 1 [file tab_suppl_ablation.tex]

\begin{table}[ht]
\makeatletter\def\@captype{table}
\centering
\adjustbox{max width=\linewidth}{%
\setlength{\tabcolsep}{2pt}
\begin{tabular}{cc*{3}{S[table-format=2.3]}l*{3}{S[table-format=2.3]}}
\toprule
  & & \multicolumn{3}{c}{Flow}
  &
  & \multicolumn{3}{c}{Intensity} \\
 \cmidrule(l{1mm}r{1mm}){3-5}
 \cmidrule(l{1mm}r{1mm}){7-9}

 Ablation & Value
 & \text{EPE$\downarrow$} & \text{AE$\downarrow$} & \text{$\%$Out$\downarrow$}
 & ~
 & \text{MSE$\downarrow$} & \text{SSIM$\uparrow$} & \text{LPIPS$\downarrow$} \\
 
\midrule
\multirow{2}{*}{\shortstack{$\lambda_2$}}

 & 0.2
 & 2.777 & 8.123 & 18.929
 &
 & 0.099 & 0.307 & 0.571 \\

 & 5.0
 & 2.34 & 9.726 & 16.417
 &
 & 0.100 & 0.309 & 0.558 \\

\midrule
\multirow{2}{*}{\shortstack{$C$}}

 & 0.1
 & 1.893 & 6.801 & 12.335
 &
 & 0.111 & 0.304 & \bnum{0.549} \\

 & 0.4
 & 1.884 & \bnum{6.422} & 12.319
 &
 & 0.101 & \bnum{0.322} & 0.557 \\

\midrule

 \multicolumn{2}{c}{\textbf{Main ($\lambda_2 = 1.0, C = 0.2$)}}
 & \bnum{1.781} & 6.439 & \bnum{11.241}
 &
 & \bnum{0.100} & 0.312 & 0.555 \\

\bottomrule
\end{tabular}
}
\caption{
\footnotesize{Results of ablation studies on $\lambda_2$ and $C$.}
\label{tab:suppl:ablation}
}
\end{table}
